# Supplementary material for: Mechanical and microscopic properties of the reversible plastic regime in a 2D jammed material
Source: arXiv:1308.6806 source file (2013-11-20)
Supplement: Supplementary file 1 [file supplemental.pdf]

# Supplementary Material for "Mechanical and microscopic properties of the reversible plastic regime in a 2D jammed material"

N. C. Keim and P. E. Arratia

## I. MOVIE CAPTIONS

`movie1.mp4, movie2.mp4, movie3.mp4` Plastic activity in each cycle at strain amplitudes $\gamma_0 = 0.01$, 0.02, and 0.04, respectively. Total (blue) and irreversible (red) local plastic activity are shown for the entire visible portion of the material, as in Fig. 2(a,b) of the paper. Vertical and horizontal axes are in units of microns.

`movie4.mp4` Close-up of material at strain amplitude $\gamma_0 = 0.02$, cycles 19–21. The cluster of T1 events in Fig. 2f of the paper is tracked. A dot is placed at the centroid of the 4 particles involved in the rearrangement, only when comparison of their positions with those at the start of the movie indicates a T1 rearrangement has occurred.

## II. DETAILS OF MATERIAL

Area fraction $\phi$ is set by the number of particles dispersed into the experimental cell, a 6 cm-diameter glass dish; positive osmotic surface pressure keeps $\phi$ uniform. We use experimental images to estimate area fraction as

$$\phi = \frac{\pi N(d_{\rm sm}^2 + d_{\rm lg}^2)}{8A_{\rm obs}}, \tag{1}$$

where $d_{\rm sm}$ and $d_{\rm lg}$ are the mean particle diameters (as measured by the manufacturer) and $A_{\rm obs}$ is the area imaged, in which $N$ particles have been identified with the same feature-identification algorithm we use for particle tracking. We measure an elastic modulus at $\phi \sim 0.36$, suggesting a jamming transition at even lower $\phi$; experiments discussed here are performed at $\phi = 0.43$, with uncertainty $\sim 0.01$. We do not expect uncertainty in $\phi$ to be a major source of error in other measurements, since we are far into the jammed regime and therefore far from any critical transition. The particles are sufficiently large that thermal motion is negligible (Péclet number $Pe \gg 1$), and we treat rearrangements as discrete, as they complete on a timescale $\sim 0.1(2\pi\omega^{-1})$, where $\omega$ is the angular frequency of driving.

To ensure reproducible interparticle forces, particles are rinsed 4 times in deionized water [1]. They are then resuspended in a water-ethanol mixture (50% by volume) to ensure dispersion at the interface. To remove polar contaminants in the oil superphase, the decane ("99+%," Acros Organics) is treated with aluminum oxide powder, which is then removed by filtration (Qualitative No. 1, Whatman). All other components are cleaned by repeated sonication and rinsing in deionized water and ethanol.

## III. IMAGING AND TRACKING OF PARTICLE POSITIONS

An important strength of our experiments is that, simultaneously with rheometry, we may image the position of nearly every particle from one side of the needle to the wall in a $\sim 2$ mm-long section of the rheometer. For proper imaging, the entire interface in the channel must be flat to within the microscope's depth of field, $\sim 10$ $\mu$m. Because the oil-water interface is pinned at the tops of the hydrophilic walls, this flatness is achieved by adjusting the water level. Whenever particle area fraction is increased by adding particle-laden aqueous suspension to the interface, an equal volume of subphase is withdrawn in order to maintain this geometry.

The material is imaged from above during shear with a long-distance microscope (K2/SC with CF–3 objective and CF amplifier, Infinity Photo-Optical) and high-speed camera (Flare 4M180, IOIndustries), with a resolution of $\sim 1.1$ $\mu$m/pixel, capturing 200 ($\gamma_0 \leq 0.02$), 400 ($\gamma_0 = 0.04$) or 600 ($\gamma_0 = 0.07$) frames per cycle at up to 80 frames/s. Particles are illuminated with diffuse light from below. We use the technique of Crocker and Grier [2] to identify particles by looking for centrally-peaked blobs in each image. Because of our backlit illumination, the largest particles have a bright optical artifact in the center, and so part of the pre-processing before particle identification is to convolve the image with an annulus, so that both small and large particles have a well-defined central maximum. With few exceptions, all particles are tracked [2, 3] for the entirety of each movie (thousands of frames) using custom, freely-available software [4].

Because we can see clearly a single layer of particles adsorbed to the needle, we know that we track nearly all particles at this boundary, and we observe that slippage is minimal. However, some particles near the wall are hidden, due to imperfect alignment of the wall with the microscope line-of-sight. We can be certain that this region does not harbor significant slippage or shear banding: the displacements of the first visible row of particles stay in proportion to the global shear strain $\gamma(t)$ over the full range of strain amplitudes $\gamma_0$, and do not creep. These displacements imply that $\sim 12$ layers of particles are hidden. Furthermore, an examination of the spatial distribution of rearrangement activity in Fig. 2(a,b) of the main paper hints at no anomalous concentration of activity in this region which would significantly affect our results.

## IV. ANALYSIS OF PARTICLE POSITIONS AND MOTION

Analysis of particle positions and motion is performed in Python, using NumPy and SciPy [5], and custom, freely-available code for the specific analyses described below [6].

### A. Characterization of static structure

Figure 1 shows the pair-correlation functions $g(|\vec{r}|)$ and $g(\vec{r})$ of the static material structure after preparation; they change very little in the course of our experiments. The structure may be described as hexatic, showing positional order on a scale of $\sim 6$ particles, as well as a preferred global hexagonal orientation, presumably set by the direction of shear. The pair correlation functions change negligibly in the course of our experiments. We note that while our particles are bidisperse, their interactions are through long-range electrostatic forces, and so the role of their size disparity is not necessarily the same as for particles with contact

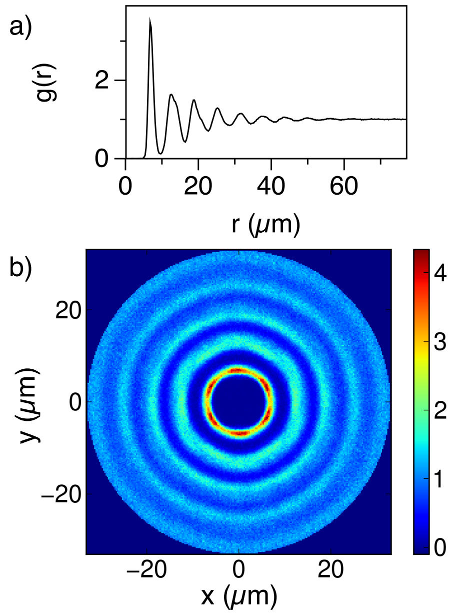


FIG. 1: **(a)** Pair correlation function $g(|\vec{r}|)$ of the material in steady state, near $\gamma(t) = \langle\gamma\rangle$, at $\gamma_0 = 0.02$. **(b)** 2-dimensional $g(\vec{r})$; the moving needle is at the $+y$ edge of the sample. The plots show that the material consists of regions of size $\sim 5$ particles with hexagonal order. The average global director is presumably set by the direction of shear motion, along the $x$ axis.

interactions.

To measure crystalline order in the environment of each particle, we compute the bond order parameter

$$\psi_6 = \frac{1}{N_r} \sum_{n=1}^{n_n} e^{i6\theta(\vec{r}_n - \vec{r}_0)} \tag{2}$$

where $n$ runs over the $N_r$ neighbors which fall within a radius $1.5a$ of the particle, and $\theta(\vec{r}_n - \vec{r}_0)$ denotes the angle that the vector from the particle to its neighbor makes with some fixed reference vector. The magnitude $|\psi_6|$ measures the extent of hexagonal crystalline ordering and has a maximum value of 1, corresponding to 6 neighbors spaced 60° apart; the phase of $\psi_6$ corresponds to the director of ordering.

### B. Analysis of particle motions

In general, a localized plastic event produces particle motions that are not affine [7]. The motion of a relative handful of particles can vastly exceed that of the rest of the system. Our analysis relies on 3 different methods to detect and describe this localized deformation of the material, sampled at times $t_1$ and $t_2$:

**Non-affine character of local particle displacements ($\mathbf{D^2_{min}}$)** Deformation localized at the single-particle level, such as rearrangement, is a breakdown of the continuum description of the material and cannot be described as an affine transformation of a neighborhood of particles. Based on the work of Falk and Langer [7], we consider the local non-affinity of

a deformation for a single particle at $\vec{r}_0$,

$$D^2(t_1, t_2) = \frac{1}{a^2 N_r} \sum_{n=1}^{n_r} \sum_i \left( r_n^i(t_1) - r_0^i(t_1) - \sum_j (\delta_{ij} + \epsilon_{ij}) \times [r_n^j(t_2) - r_0^j(t_2)] \right)^2 . \qquad (3)$$

$n$ runs over the nearest 2 "shells" of neighboring particles, out to the second trough in the pair correlation function $g(|\vec{r}|)$ (Fig. 1a), or $\sim 2.5a$, where $a$ is the position of the first peak of $g(|\vec{r}|)$ — the typical separation between particles. $i$ and $j$ refer to spatial coordinates, so that $\epsilon_{ij}$ are elements of an affine deformation tensor which is applied to the neighborhood of the particle in question, with $\vec{r}_0$ at the origin. $D^2$ is thus the sum, in quadrature, of the difference between the transformed positions and the actual positions, normalized by the number of neighbors considered $N_r$, and the interparticle spacing $a$. We then use a least-squares optimization algorithm to find the $\epsilon_{ij}$ that minimize $D^2$, yielding a $D^2_{\rm min}(t_1, t_2)$ for nearly every particle in the system between any two instants. To reduce the presence of spuriously high $D^2_{\rm min}$ due to noise in locating particles, we also consider the particle positions in the frames immediately before and after $t_1$ and $t_2$, and take the median position in $x$ and $y$. (This is not done for the hysteresis computations, which intrinsically consider many frames.) Finally, due to shearing, the boundary of tracked particles is not rectilinear at the left and right edges of the frame, making some $D^2_{\rm min}$ calculations unreliable. Therefore 100 $\mu$m on each end of the image (measured along the length of the needle) are generally excluded from calculations of global quantities (*e.g.* $\langle D^2_{\rm min} \rangle$).

**Topological rearrangements (T1 events)** Strain localization also corresponds to rearrangements, in which particles lose some nearest neighbors and gain others. In 2 dimensions, such changes to the topology of the packing may be atomically discretized as T1 rearrangements [8]. Each T1 rearrangement is associated with 4 particles — one pair that are nearest neighbors before the event, and an associated pair that become nearest neighbors afterward. The nearest-neighbor relationships are computed by Delaunay triangulation [9] for the entire packing at times $t_0$ and $t_1$, and then compared. We remove the least significant events by requiring both that the topology be altered and that

$$-\frac{(r^0_{12} - r^1_{12})(r^0_{34} - r^1_{34})}{(r^0_{12} + r^1_{12})(r^0_{34} + r^1_{34})} \geq \delta_{\rm T1}. \qquad (4)$$

where $r_{12}$ and $r_{34}$ are the separations of the particle pairs in the T1 event and the superscripts 0 and 1 denote the times at which particle positions are compared. In the analysis we present below, $\delta_{\rm T1} = 0.005$. Lowering this threshold to $10^{-4}$ effectively adds a noise floor of $\sim 10$ events per cycle to all movies, suggesting that $\delta_{\rm T1} = 0.005$ is close to a noise floor created by random error in particle tracking.

**Local relative displacements** Finally, to analyze particle trajectories in space, we need to subtract from each particle's motion the coarse-grained displacements that are due to bulk shear deformation, or to other factors such as small vibrations of the microscope. For a single particle at $\vec{r}_0$ between times $t_0$ and $t_1$, we do this by subtracting the mean displacement of all particles that are within distance $R_{\rm coarse}$ of $\vec{r}_0$ at time $t_0$. $R_{\rm coarse} = 10a$ in the main paper, except in Fig. 2e of the main paper, where $R_{\rm coarse} = 40a$ because of larger region shown. Local relative displacements are not computed within $R_{\rm coarse}$ of the edges of the region of visible particles.

### C. Rheometry

We model the response of the interfacial stress rheometer (ISR) with the following equation of motion [10] for the needle position $x$:

$$m\ddot{x} = AI_{\text{drive}} - kx - d\dot{x} - F_s \quad (5)$$

where $m$ is the needle mass, $AI_{\text{drive}}$ is the force from the computer-controlled driving current, $k$ is the spring constant for the central potential of the Helmholtz field, $d$ represents drag from the bulk fluid, and $F_s$ is due to any material adsorbed at the surface. If $m$ is known, the values of $a$, $k$, and $d$ may be determined by applying a sinusoidal $I_{\text{drive}}$ on a clean interface at a range of frequencies, allowing computation of $F_s(t)$ from $x(t)$, and so permitting measurement of the oscillatory rheology of a material. We obtain $x(t)$ when the interface is clean by tracking small irregularities on the surface of the needle; tests show that this response is linear with respect to $I_{\text{drive}}$. When particles are present, the needle position is measured by tracking the first $\sim 5$ layers of particles at the needle (tracking method described above), which we validate visually by observing irregularities on the surface of the needle.

Once particles have been added to the interface, rheometry is performed by using a fast Fourier transform to determine the phase and amplitude of the needle response near the driving frequency, then applying a linear correction for subphase drag and needle mass, based on Eq. 5 [10]. All measurements in the present work are in the steady state and at 0.1 or 0.2 Hz; we have observed that under these experimental conditions, oscillatory rheology varies little with frequency.

For the linear correction method to be accurate, and for shear stress to be nearly uniform throughout the material, the mechanical response of the interface must be decoupled from that of the bulk fluids above and below [11]. This decoupling is characterized by the Boussinesq number $Bq = |\eta_i^*|/\eta_b a_N$, the dimensionless ratio of interfacial and bulk stresses, where $\eta_i^*$ is the complex interfacial viscosity, $\eta_b$ is the bulk fluid viscosity, and $a_N$ is the diameter of the needle [10, 11]. Here $Bq \sim 100$, so that to a good approximation we measure only the interfacial rheology. We can similarly consider how the nominal shear stress within the material compares with viscous stress from without; here the length scale for computing $Bq$ is of the order of a particle diameter, and thus $Bq \gg 1$ in that case also. This means that effectively, stress is applied to the material at its boundaries only.

A further condition for proper operation applies to interfacial materials with a yield stress: if the needle is much shorter than the channel, unyielded material forms "plugs" at the ends of the needle, so that when material inside the gap is fluidized by shear, it shows circulation instead of near-uniform shear. In our experiments, the needle (length 22 mm) is slightly longer than the channel (width 3.5 mm, length 18 mm), and the device is at least $\sim 75$ channel widths away from the walls of the cell, so that unsheared material has minimal influence on our measurement.


[1] B. J. Park, J. Vermant, and E. M. Furst, Soft Matter **6**, 5327 (2010).

[2] J. C. Crocker and D. G. Grier, J. Colloid Interf. Sci. **179**, 298 (1996).

[3] T. A. Caswell, URL `https://github.com/tacaswell/trackpy`.

[4] N. C. Keim, URL `https://github.com/nkeim/runtrackpy`.

[5] E. Jones, T. Oliphant, P. Peterson, et al., *SciPy: Open source scientific tools for Python* (2001–), URL http://www.scipy.org/.

[6] N. C. Keim, URL https://github.com/nkeim/philatracks.

[7] M. L. Falk and J. S. Langer, Phys. Rev. E **57**, 7192 (1998).

[8] D. Weaire and N. Rivier, Contemp. Phys. **25**, 59 (1984).

[9] C. B. Barber, D. P. Dobkin, and H. Huhdanpaa, ACM Trans. Math. Softw. **22**, 469 (1996).

[10] C. F. Brooks, G. G. Fuller, C. W. Frank, and C. R. Robertson, Langmuir **15**, 2450 (1999).

[11] S. Reynaert, C. F. Brooks, P. Moldenaers, J. Vermant, and G. G. Fuller, J. Rheol. **52**, 261 (2008).
